# Supplementary material for: Mapping spiral waves and other radial features in Saturn's rings
Source: arXiv:1708.03702 ancillary file (2017-08-11)
Supplement: Supplementary file 1 [file ringsres7_AppendixA.pdf]

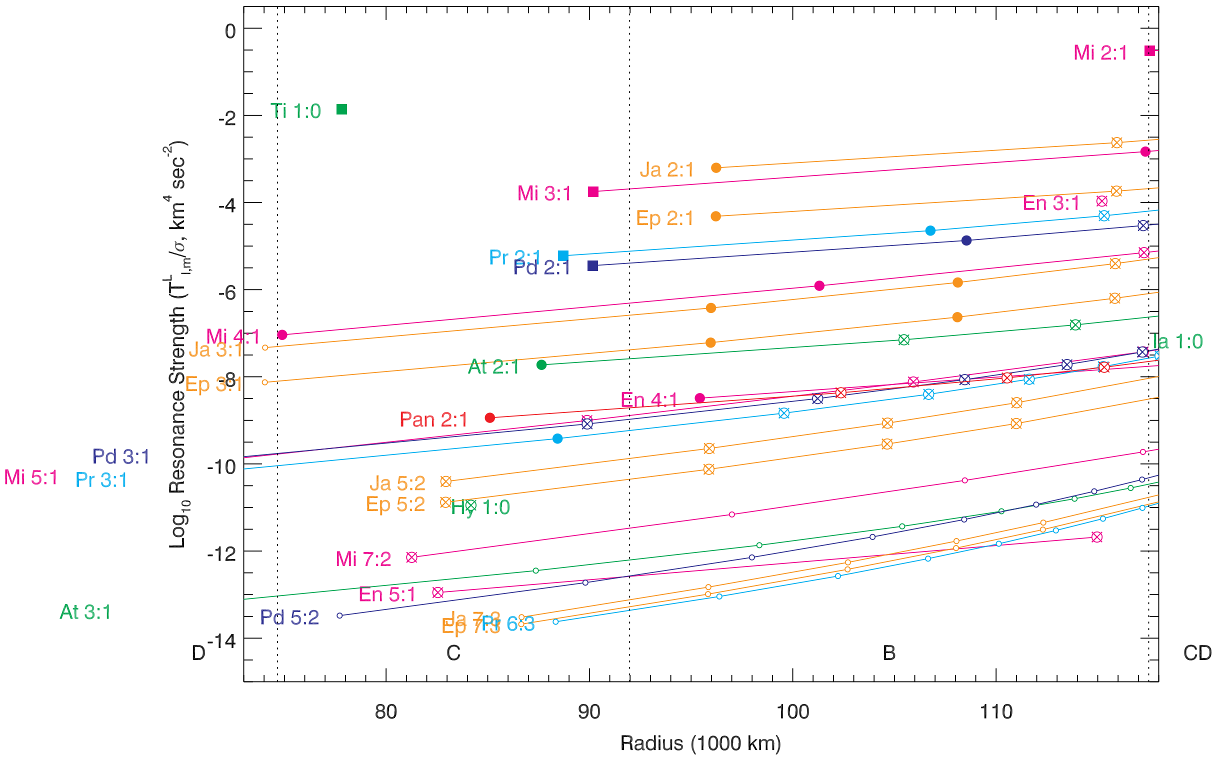


Figure A1: Resonance atlas for a portion of Saturn's rings, like that of Fig. 19 but focusing on the B and C rings.

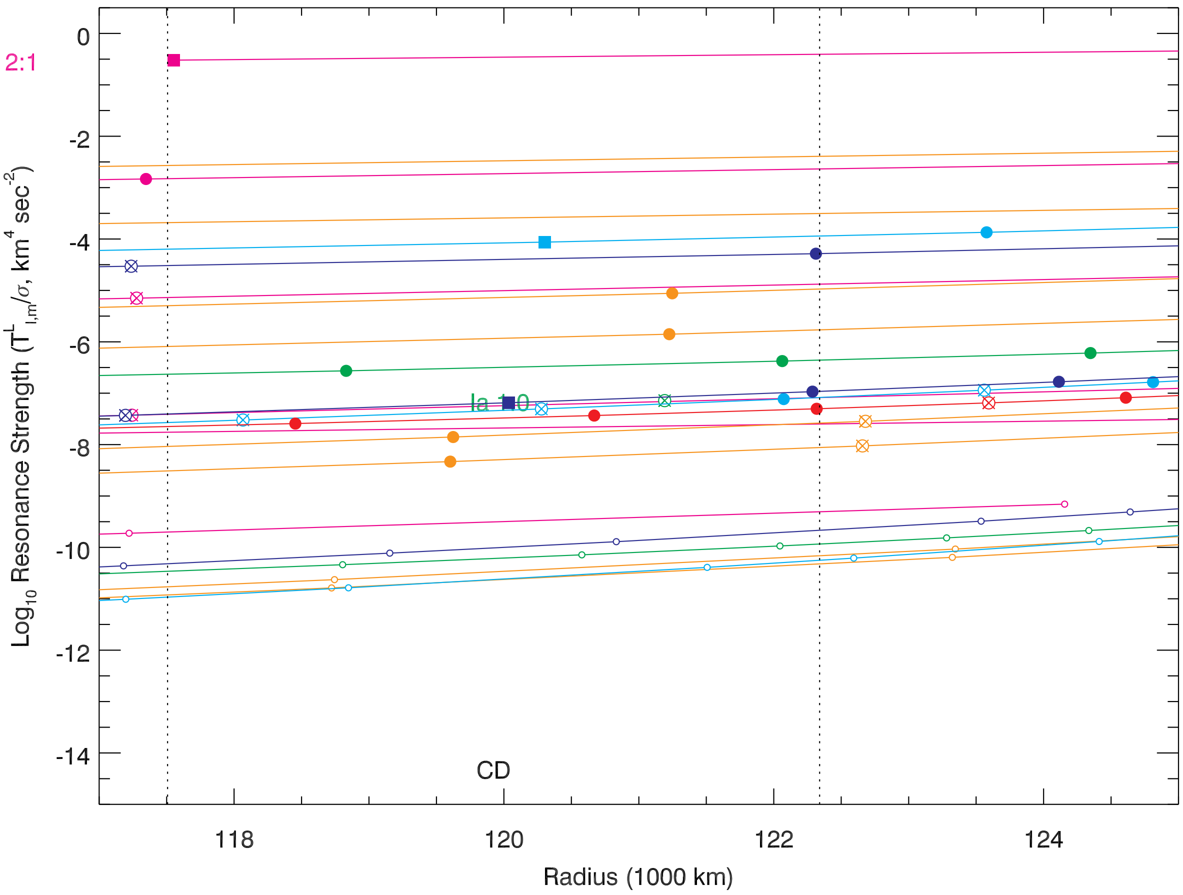


Figure A2: Resonance atlas for a portion of Saturn's rings, like that of Fig. 19 but focusing on the Cassini Division and inner A ring.

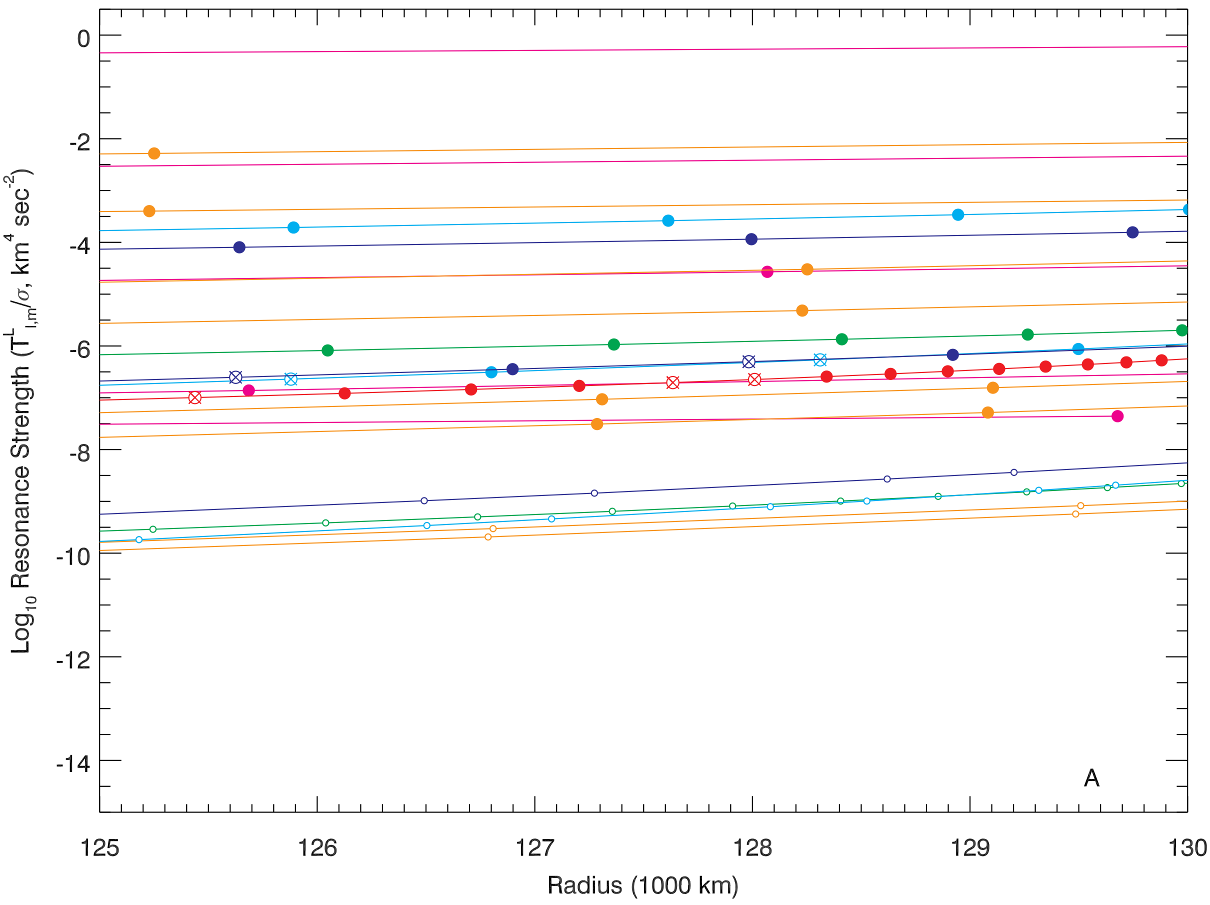


Figure A3: Resonance atlas for a portion of Saturn's rings, like that of Fig. 19 but focusing on the inner-middle A ring.

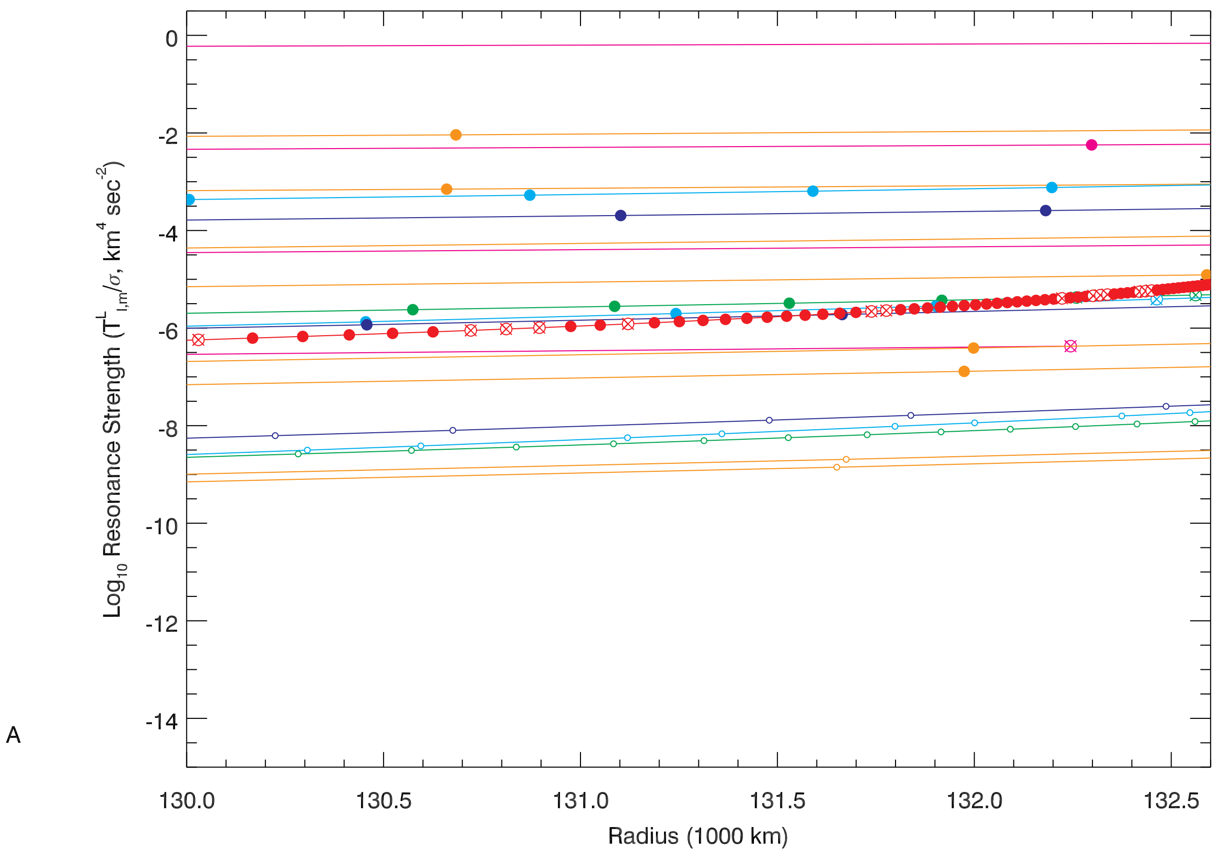


Figure A4: Resonance atlas for a portion of Saturn's rings, like that of Fig. 19 but focusing on the middle A ring.

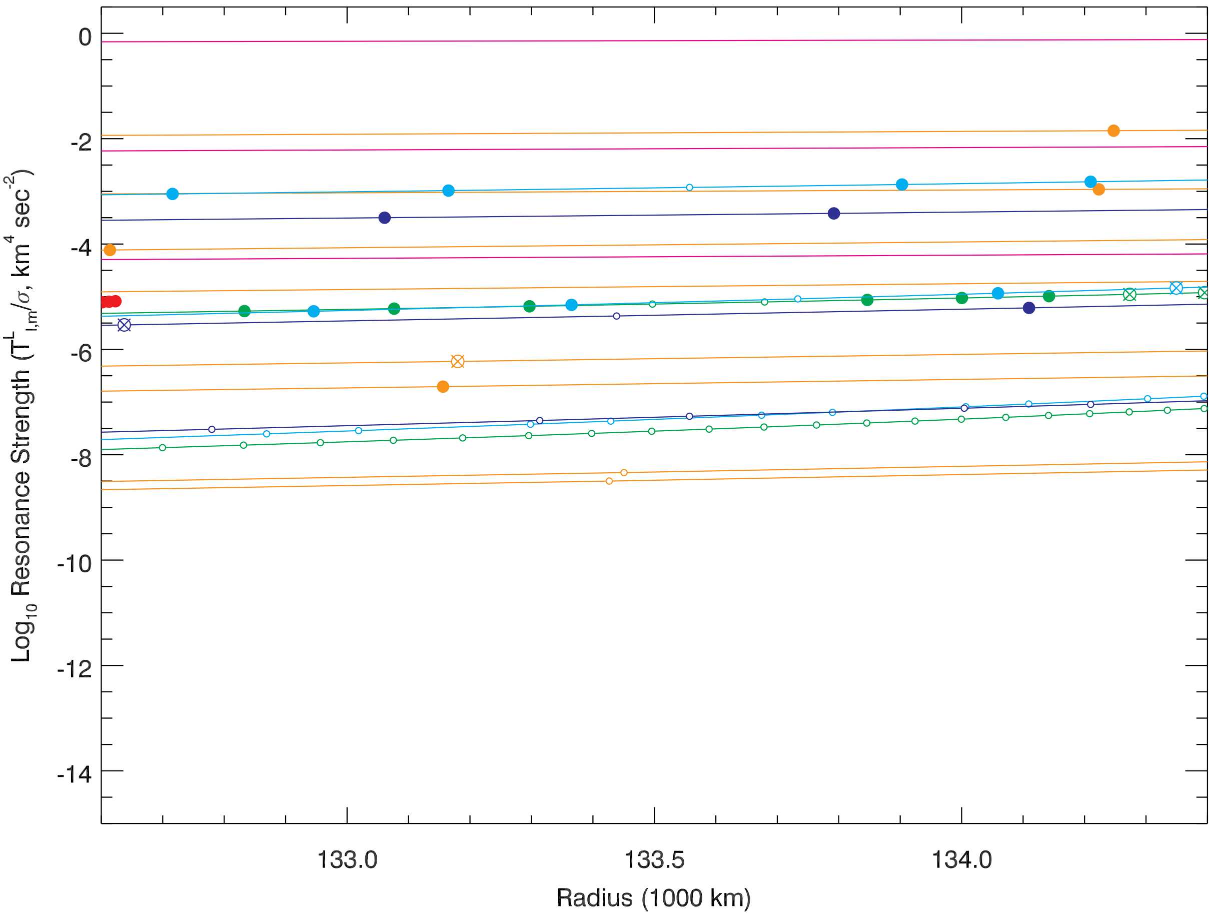


Figure A5: Resonance atlas for a portion of Saturn's rings, like that of Fig. 19 but focusing on the outer-middle A ring.

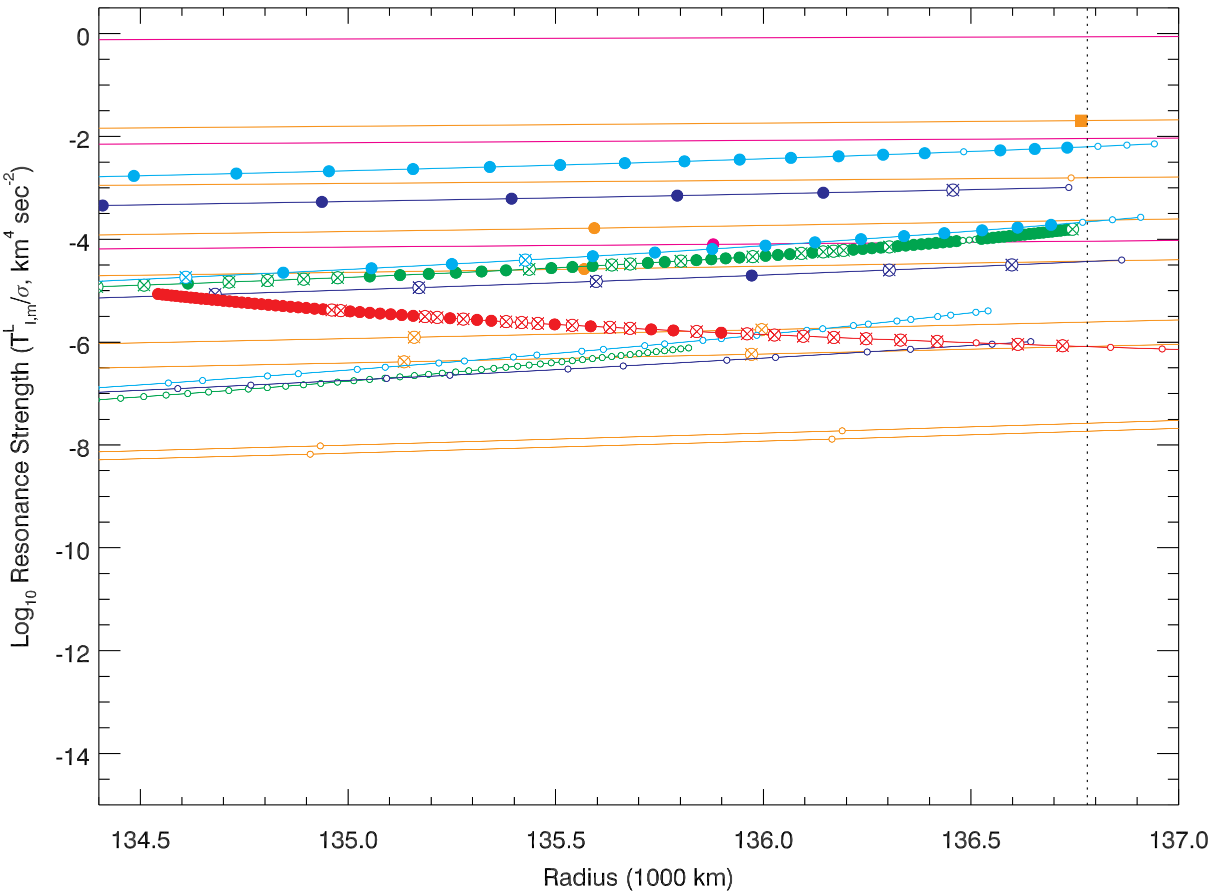


Figure A6: Resonance atlas for a portion of Saturn's rings, like that of Fig. 19 but focusing on the outer A ring.
